# Supplementary material for: Alignment of non-spherical active particles in chaotic flows
Source: arXiv:1909.02458 ancillary file (2019-09-05)
Supplement: Supplementary file 1 [file supplements.pdf]

# Supplemental material for 'Alignment of spheroidal self-propelled particles swimming in turbulent flows'

M. Borgnino[1], K. Gustavsson[2], F. De Lillo[1], G. Boffetta[1], M. Cencini[3], and B. Mehlig[2]
[1]*Dipartimento di Fisica and INFN, Universita di Torino, via P. Giuria 1, 10125 Torino, Italy*
[2]*Department of Physics, Gothenburg University, SE-41296 Gothenburg, Sweden and*
[3]*Istituto dei Sistemi Complessi, CNR, via dei Taurini 19, 00185 Rome, Italy and INFN, sez. Roma2 "Tor Vergata"*

**Contents**

**I. Model** 2
A. Connection between statistical model parameters and turbulent flow characteristics 2

**II. Trajectory expansion for $\langle \boldsymbol{u} \cdot \boldsymbol{n} \rangle$** 3
A. Trajectory expansion to order $O(\mathrm{Ku}^2)$ 3
B. Correlation functions 4
C. Results 5

**III. Higher moments $\langle (\boldsymbol{u}(\boldsymbol{x}_t, t) \cdot \boldsymbol{n}_t)^p \rangle$** 6

**IV. Alignment with vorticity** 7

**V. Average alignment for turbulent flows** 7

**References** 8

This Supplemental Material contains a summary of the statistical-model derivation of Eqs. (4,5) and (7) in the Letter, as well as a discussion of how these results apply to turbulent flows [Eq. (6) in the Letter]. For the sake of completeness, the previously known alignment with vorticity (See Refs.[14,31] of the Letter) is also briefly discussed.

The material is organized as follows. In Section I, we briefly describe the statistical model and how its parameters connect to the turbulent flow. Section II explains how to calculate $\langle \boldsymbol{u}\cdot\boldsymbol{n}\rangle$ using a systematic expansion in powers of the Kubo number, Ku. Section III gives the corresponding results for the second moment, and for the distribution of $\boldsymbol{u}(\boldsymbol{x}_t,t)\cdot\boldsymbol{n}_t$ to lowest order in Ku. Section IV discusses the alignment of $\boldsymbol{n}_t$ with fluid vorticity, $\boldsymbol{\omega}(\boldsymbol{x}_t,t)=\boldsymbol{\nabla}\wedge\boldsymbol{u}(\boldsymbol{x}_t,t)$. Finally, in Section V we show how to estimate the average alignment for turbulence. We obtain the same parameter dependence as in the statistical model, namely that the average alignment is proportional to the product of the shape factor $\Lambda$ and the swimming speed $v_{\rm s}$, and we give a heuristic argument for the numerical prefactor.

## I. MODEL

We consider microswimmers much smaller than the Kolmogorov length $\eta$ of the turbulent flow. Therefore, the swimmers interact with the turbulent velocity fluctuations in the dissipative range. We use a statistical model [S4] for these fluctuations, representing the turbulent velocity $\boldsymbol{u}(\boldsymbol{x},t)$ by an incompressible, homogeneous, isotropic Gaussian random function with correlation length $\ell_f$ and correlation time $\tau_f$. We follow Ref. [S4] and write in three spatial dimensions $\boldsymbol{u}(\boldsymbol{x},t)=\frac{1}{\sqrt{6}}\boldsymbol{\nabla}\wedge\boldsymbol{A}(\boldsymbol{x},t)$. The components of the field $\boldsymbol{A}(\boldsymbol{x},t)$ are Gaussian random functions with zero mean and correlation functions

$$\langle A_i(\boldsymbol{x},t)A_j(\boldsymbol{x}',t')\rangle=\delta_{ij}\ell_f^2u_f^2\exp\Big(-\frac{|\boldsymbol{x}-\boldsymbol{x}'|^2}{2\ell_f^2}-\frac{|t-t'|}{\tau_f}\Big)\,, \tag{S1}$$

so that $u_f^2=\langle|\boldsymbol{u}|^2\rangle$. The $\boldsymbol{x}$-dependence of the functions $A_j(\boldsymbol{x},t)$ is constructed as a superposition of Fourier modes with random coefficients, so that the spatial correlation function of $\boldsymbol{A}(\boldsymbol{x},t)$ is Gaussian. Its time dependence is obtained from Ornstein-Uhlenbeck processes, resulting in exponentially decaying time correlations. A two-dimensional statistical model can be defined in an analogous way, by writing $\boldsymbol{u}(\boldsymbol{x},t)=\frac{1}{\sqrt{2}}\boldsymbol{\nabla}\wedge A(\boldsymbol{x},t)\hat{\rm e}_3$. Details are given in Ref. [S4]. The parameters $\ell_f$, $\tau_f$, and $u_f$ can be combined into the dimensionless Kubo number

$$\mathrm{Ku}=\frac{u_f\tau_f}{\ell_f}\,, \tag{S2}$$

a measure of the persistence of the flow. Large values of Ku correspond to a flow that is persistent in time, whereas the limit $\mathrm{Ku}\to 0$ describes velocity fluctuations that are white noise in time. In this limit the statistical model is similar to smooth Kraichnan flows [S2].

### A. Connection between statistical model parameters and turbulent flow characteristics

The length and time scales of the statistical model are related to the Kolmogorov scales as follows. The Kolmogorov time is defined as $\tau_\eta=(2\langle\mathrm{Tr}\,\mathbb{S}\mathbb{S}^{\sf T}\rangle)^{-1/2}$ where $\mathbb{S}$ is the strain-rate matrix. Evaluating the average in the statistical model yields

$$\frac{\tau_f}{\tau_\eta}=\sqrt{d+2}\,\mathrm{Ku}\,, \tag{S3}$$

where $d\geq 2$ is the spatial dimension in which the statistical model is analyzed.

The length scale $\ell_f$ is matched to the Kolmogorov length $\eta_K$ as follows [S6]. The alignment is driven by the fluid-velocity gradients, as Eq. (6) in the Letter shows. Specifically, the alignment is expressed in terms of a time integral over the strain correlation evaluated at zero spatial separation, averaged over Lagrangian trajectories. In our model, this local property of the fluid-velocity gradients is related to $\ell_f$ by $\ell_f^2=\langle(\partial_1u_1)^2\rangle/\langle u_1^2\rangle$. In turbulence, this expression defines the Taylor scale, $\lambda$ [S1, S3]. Consequently, the spatial correlation length in the statistical model should be identified with the Taylor length in turbulence. The latter is related to the Kolmogorov length $\eta$ by

$$\lambda=\eta C\mathrm{Re}_\lambda^{1/2}$$

where $\mathrm{Re}_\lambda$ is the Taylor-scale Reynolds number [S3], and where $C$ is a numerical constant of order unity [S1]. This implies that

$$\frac{\ell_f}{\eta}=C\mathrm{Re}_\lambda^{1/2}\,. \tag{S4}$$

Eqs. (S3) and (S4) define how the statistical-model parameters map to those of the DNS.

Let us discuss the dimensionless parameters of the statistical model. The equations of motion for a small swimmer are given by Eqs. (1) and (2) in the Letter. We use $t = t'\tau_f$, $\boldsymbol{x} = \boldsymbol{x}'\ell_f$, $\boldsymbol{u} = \boldsymbol{u}'u_f$ to de-dimensionalize Eqs. (1) and (2):

$$\dot{\boldsymbol{x}}_t = \mathrm{Ku}\,\boldsymbol{u}(\boldsymbol{x}_t, t) + \Phi_\mathrm{s}\,\boldsymbol{n}_t\,, \tag{S5a}$$

$$\dot{\boldsymbol{n}}_t = \mathrm{Ku}\,[\mathbb{B}(\boldsymbol{x}_t, t)\boldsymbol{n}_t - (\boldsymbol{n}_t\cdot\mathbb{B}(\boldsymbol{x}_t, t)\boldsymbol{n}_t)\boldsymbol{n}_t] \equiv \mathrm{Ku}\,\boldsymbol{J}_t\,, \tag{S5b}$$

where $\mathbb{B} = \mathbb{O} + \Lambda\mathbb{S}$. So there are two dimensionless parameters that determine the statistical-model dynamics, the Kubo number and the dimensionless swimming speed

$$\Phi_\mathrm{s} = \frac{v_\mathrm{s}\tau_f}{\ell_f} \tag{S6}$$

in the statistical model. This parameter is related in the following way to the parameter $\Phi$ in the main text of the Letter:

$$\Phi = \Phi_\mathrm{s}\,\frac{\tau_\eta}{\tau_f}\frac{\ell_f}{\eta} = \Phi_\mathrm{s}\,\frac{C\sqrt{\mathrm{Re}_\lambda}}{\sqrt{d+2}\,\mathrm{Ku}}\,. \tag{S7}$$

Eq. (S7) predicts how the DNS results depend on the Reynolds number of the turbulent flow: when plotted as a function of $\Phi/\sqrt{\mathrm{Re}_\lambda}$, any dimensionless variable should be independent of the Reynolds number $\mathrm{Re}_\lambda$. Noticing that the Taylor scale can equivalently be rewritten as $\lambda = Cu_{rms}\tau_\eta$, one can recognize that $\Phi_s = v_s/(Cu_\mathrm{rms})$, in other terms the prediction of the statistical model is that the result should not depend on $Re_\lambda$ provided that the swimming speed remains the same with respect to the large scale velocity of turbulence, this observation matches previous results obtained comparing the statistical model for gyrotactic swimmers in turbulence (see Ref.[19] of the Letter).

## II. TRAJECTORY EXPANSION FOR $\langle \boldsymbol{u}\cdot\boldsymbol{n}\rangle$

### A. Trajectory expansion to order $O(\mathrm{Ku}^2)$

We solve the equations of motion Eq. (S5a) implicitly as

$$\boldsymbol{x}_t = \boldsymbol{x}_0 + \int_0^t \mathrm{d}t_1[\mathrm{Ku}\,\boldsymbol{u}(\boldsymbol{x}_{t_1}, t_1) + \Phi_\mathrm{s}\,\boldsymbol{n}_{t_1}]\,, \tag{S8a}$$

$$\boldsymbol{n}_t = \boldsymbol{n}_0 + \mathrm{Ku}\int_0^t \mathrm{d}t_1\boldsymbol{J}_{t_1}\,, \tag{S8b}$$

with initial conditions $\boldsymbol{x}_0$ and $\boldsymbol{n}_0$. The dimensionless tumbling rate $\mathrm{Ku}\,\boldsymbol{J}_t$ is defined in Eq. (S5b). In order to determine $\langle \boldsymbol{u}(\boldsymbol{x}_t, t)\cdot\boldsymbol{n}_t\rangle$ we need to compute

$$\langle \boldsymbol{u}(\boldsymbol{x}_t, t)\cdot\boldsymbol{n}_t\rangle = \langle \boldsymbol{u}(\boldsymbol{x}_t, t)\cdot\boldsymbol{n}_0\rangle + \mathrm{Ku}\int_0^t \mathrm{d}t_1\langle \boldsymbol{u}(\boldsymbol{x}_t, t)\cdot\boldsymbol{J}_{t_1}\rangle\,. \tag{S9}$$

The averages are over velocity fluctuations. To evaluate this average in the integral on the r.h.s. of Eq. (S9), we expand the dynamics to the desired order in Ku. Then we take the average, expressing the moments of $\boldsymbol{u}(\boldsymbol{x}_t, t)\cdot\boldsymbol{n}_t$ in terms of correlation functions of $\boldsymbol{u}(\boldsymbol{x}_t, t)$ and its gradients. Specifically, we decompose $\boldsymbol{x}_t = \boldsymbol{x}_t^{(\mathrm{d})} + \delta\boldsymbol{x}_t$, where $\boldsymbol{x}_t^{(\mathrm{d})} = \boldsymbol{x}_0 + \Phi_\mathrm{s}\,\boldsymbol{n}_0 t$ is the deterministic solution of the problem (for $\mathrm{Ku} = 0$), and $\delta\boldsymbol{x}_t$ represents fluctuations around this deterministic solution. Iterating this procedure we obtain successively improved estimates for the trajectories $\boldsymbol{x}_t$. It was shown in Ref. [S5] that this generates an expansion of the solution in powers of Ku.

Here we compute $\langle \boldsymbol{u}(\boldsymbol{x}_t, t)\cdot\boldsymbol{n}_t\rangle$ to order $O(\mathrm{Ku}^2)$. To this order we have:

$$\delta\boldsymbol{x}_t = \mathrm{Ku}\int_0^t \mathrm{d}t_1\,[\boldsymbol{u}(\boldsymbol{x}_{t_1}, t_1) + \Phi_\mathrm{s}(t-t_1)\boldsymbol{J}_{t_1}] + O(\mathrm{Ku}^2)\,. \tag{S10}$$

Expanding $\boldsymbol{u}(\boldsymbol{x}_t,t)$ to first order in $\delta\boldsymbol{x}_t$ gives $\boldsymbol{u}(\boldsymbol{x}_t,t)=\boldsymbol{u}(\boldsymbol{x}_t^{(\mathrm{d})},t)+\mathbb{A}(\boldsymbol{x}_t^{(\mathrm{d})},t)\delta\boldsymbol{x}_t$. Here $\mathbb{A}$ is the matrix of fluid-velocity gradients with entries $A_{ij}=\partial_j u_i$. Inserting this expansion into Eq. (S9) and using Eq. (S10) gives

$$\begin{aligned}\langle \boldsymbol{n}_t\cdot\boldsymbol{u}(\boldsymbol{x}_t,t)\rangle &= \underbrace{\langle \boldsymbol{n}_0\cdot\boldsymbol{u}(\boldsymbol{x}_t^{(\mathrm{d})},t)\rangle}_{=0} + \mathrm{Ku}\int_0^t \mathrm{d}t_1 \langle \boldsymbol{J}_{t_1}\cdot\boldsymbol{u}(\boldsymbol{x}_t^{(\mathrm{d})},t)\rangle \\ &+\mathrm{Ku}\underbrace{\langle \boldsymbol{n}_0\cdot\mathbb{A}(\boldsymbol{x}_t^{(\mathrm{d})},t)\int_0^t \mathrm{d}t_1 \boldsymbol{u}(\boldsymbol{x}_{t_1}^{(\mathrm{d})},t_1)\rangle}_{=0\ \text{(homogeneity+incompressibility)}} + \mathrm{Ku}\,\Phi_\mathrm{s}\langle \boldsymbol{n}_0\cdot\mathbb{A}(\boldsymbol{x}_t^{(\mathrm{d})},t)\int_0^t \mathrm{d}t_1 (t-t_1)\boldsymbol{J}_{t_1}\rangle \end{aligned} \tag{S11}$$

with

$$\boldsymbol{J}_t = \mathbb{B}(\boldsymbol{x}_t^{(\mathrm{d})},t)\boldsymbol{n}_0 - \big(\boldsymbol{n}_0\cdot\mathbb{B}(\boldsymbol{x}_t^{(\mathrm{d})},t)\boldsymbol{n}_0\big)\boldsymbol{n}_0 + O(\mathrm{Ku})\,. \tag{S12}$$

This result expresses the first moment of $\boldsymbol{u}(\boldsymbol{x}_t,t)\cdot\boldsymbol{n}_t$ in terms of time integrals over the correlation functions $\langle u_i(\boldsymbol{r}_t^{(\mathrm{d})},t)B_{i'j'}(\boldsymbol{r}_{t_1}^{(\mathrm{d})},t_1)\rangle$ and $\langle A_{ij}(\boldsymbol{r}_t^{(\mathrm{d})},t)B_{i'j'}(\boldsymbol{r}_{t_1}^{(\mathrm{d})},t_1)\rangle$.

### B. Correlation functions

The form of the velocity correlations for an incompressible, isotropic, homogeneous velocity field is determined by the symmetry properties of this field:

$$\langle u_i(\boldsymbol{R},t)u_j(\boldsymbol{0},0)\rangle = \left[\frac{1}{d-1}RC_\parallel'(R,t)+C_\parallel(R,t)\right]\delta_{ij} - \frac{1}{d-1}\frac{R_iR_j}{R}C_\parallel'(R,t) \tag{S13}$$

where $R=|\boldsymbol{R}|$ and $C_\parallel(R,t)\equiv\langle(\boldsymbol{u}(\boldsymbol{R},t)\cdot\hat{\boldsymbol{R}})(\boldsymbol{u}(\boldsymbol{0},0)\cdot\hat{\boldsymbol{R}})\rangle$. In Eq. (S13), $C_\parallel'(R,t)$ denotes the derivative of $C_\parallel(R,t)$ w.r.t. $R$.

We compute the correlation functions $\langle u_i(\boldsymbol{r}_t^{(\mathrm{d})},t)B_{i'j'}(\boldsymbol{r}_{t_1}^{(\mathrm{d})},t_1)\rangle$ and $\langle A_{ij}(\boldsymbol{r}_t^{(\mathrm{d})},t)B_{i'j'}(\boldsymbol{r}_{t_1}^{(\mathrm{d})},t_1)\rangle$ by expressing them in terms of the elementary correlations

$$\begin{aligned}\langle u_i(\boldsymbol{R},t)u_i(\boldsymbol{0},0)\rangle &= RC_\parallel'(R,t)+dC_\parallel(R,t)\\ \langle u_i(\boldsymbol{R},t)u_j(\boldsymbol{0},0)\rangle n_{0,i}n_{0,j} &= \frac{1}{d-1}\sin^2\theta RC_\parallel'(R,t)+C_\parallel(R,t)\,.\end{aligned} \tag{S14}$$

Here $\theta$ is the angle between $\boldsymbol{n}_0$ and $\boldsymbol{R}$, and summation over repeated indices is implied. The first step is to evaluate the following correlation functions:

$$\begin{aligned}\langle B_{ik}(\boldsymbol{R},t)u_j(\boldsymbol{0},0)\rangle &= \frac{\Lambda+1}{2}\partial_k\langle u_i(\boldsymbol{R},t)u_j(\boldsymbol{0},0)\rangle + \frac{\Lambda-1}{2}\partial_i\langle u_k(\boldsymbol{R},t)u_j(\boldsymbol{0},0)\rangle\\ \langle B_{ik}(\boldsymbol{R},t)A_{jl}(\boldsymbol{0},0)\rangle &= -\frac{\Lambda+1}{2}\partial_k\partial_l\langle u_i(\boldsymbol{R},t)u_j(\boldsymbol{0},0)\rangle - \frac{\Lambda-1}{2}\partial_i\partial_l\langle u_k(\boldsymbol{R},t)u_j(\boldsymbol{0},0)\rangle\end{aligned} \tag{S15}$$

where we used that $\mathbb{B}=\frac{\Lambda+1}{2}\mathbb{A}+\frac{\Lambda-1}{2}\mathbb{A}^\mathsf{T}$. Contracting the expressions in Eq. (S15) with suitable combinations of $\boldsymbol{n}$ and Kronecker deltas, using homogeneity and incompressibility, and finally inserting the expressions from Eq. (S14), we obtain

$$\begin{aligned}&\langle B_{ij}(\boldsymbol{R},t)u_i(\boldsymbol{0},0)\rangle n_{0,j} = \frac{\Lambda+1}{2}\partial_j\langle u_i(\boldsymbol{R},t)u_i(\boldsymbol{0},0)\rangle n_{0,j} = \frac{\Lambda+1}{2}\frac{\boldsymbol{n}_0\cdot\boldsymbol{R}}{R}\frac{\partial}{\partial R}\langle u_i(\boldsymbol{R},t)u_i(\boldsymbol{0},0)\rangle\\ &= \frac{\Lambda+1}{2}\frac{\boldsymbol{n}_0\cdot\boldsymbol{R}}{R}((d+1)C_\parallel'(R,t)+RC_\parallel''(R,t))\\ &\langle B_{jk}(\boldsymbol{R},t)u_i(\boldsymbol{0},0)\rangle n_{0,j}n_{0,k}n_{0,i} = \Lambda\partial_k\langle u_j(\boldsymbol{R},t)u_i(\boldsymbol{0},0)\rangle n_{0,j}n_{0,k}n_{0,i}\\ &= \Lambda\left[\frac{\boldsymbol{n}_0\cdot\boldsymbol{R}}{R}\frac{\partial}{\partial R}-\frac{\sin\theta}{R}\frac{\partial}{\partial\theta}\right]\langle u_j(\boldsymbol{R},t)u_i(\boldsymbol{0},0)\rangle n_{0,j}n_{0,i} = \Lambda\frac{\boldsymbol{n}_0\cdot\boldsymbol{R}}{R}C_\parallel'(R,t)\\ &\langle B_{jk}(\boldsymbol{R},t)A_i{}^j(\boldsymbol{0},0)\rangle n_{0,i}n_{0,k} = -\frac{\Lambda-1}{2}\partial_j\partial^j\langle u_k(\boldsymbol{R},t)u_i(\boldsymbol{0},0)\rangle n_{0,i}n_{0,k}\\ &= -\frac{\Lambda-1}{2}\frac{1}{R}((d+1)C_\parallel'(R,t)+RC_\parallel''(R,t))\end{aligned}$$

$$
\begin{aligned}
&\langle B_{kl}(\boldsymbol{R},t)A_{ij}(\boldsymbol{0},0)\rangle n_{0,i}n_{0,j}n_{0,k}n_{0,l} = -\Lambda\partial_l\partial_j\langle u_k(\boldsymbol{R},t)u_i(\boldsymbol{0},0)\rangle n_{0,i}n_{0,j}n_{0,k}n_{0,l} \\
&= -\Lambda\left[\cos^2\theta\frac{\partial^2}{\partial R^2} + \frac{\sin^2\theta}{R}\frac{\partial}{\partial R} + \frac{\sin(2\theta)}{R^2}\frac{\partial}{\partial\theta} - \frac{\sin(2\theta)}{R}\frac{\partial^2}{\partial R\partial\theta} + \frac{\sin^2\theta}{R^2}\frac{\partial^2}{\partial\theta^2}\right]\langle u_k(\boldsymbol{R},t)u_i(\boldsymbol{0},0)\rangle n_{0,i}n_{0,j}n_{0,k}n_{0,l} \\
&= -\Lambda C_\parallel''(R,t)\,.
\end{aligned}
$$

Here we have set $\sin\theta = 0$, because in the following we evaluate these correlation functions along deterministic trajectories. This means that $\boldsymbol{R} \propto \boldsymbol{n}_0 t$, i.e. $\sin\theta = 0$.

In a second step we use these results to obtain the following correlations between the flow and $\boldsymbol{J}$ evaluated to lowest order in Ku:

$$
\begin{aligned}
\langle \boldsymbol{u}(\boldsymbol{x}_t^{(\mathrm{d})},t)\cdot\boldsymbol{J}_{t_1}\rangle &= \langle B_{ij}(\boldsymbol{x}_{t_1}^{(\mathrm{d})},t_1)u_i(\boldsymbol{x}_t^{(\mathrm{d})},t)\rangle n_{0,j} - \langle B_{jk}(\boldsymbol{x}_{t_1}^{(\mathrm{d})},t_1)u_i(\boldsymbol{x}_t^{(\mathrm{d})},t)\rangle n_{0,j}n_{0,k}n_{0,i} \\
&= \frac{\boldsymbol{n}_0\cdot\boldsymbol{R}}{2R}\Big[[(d+1)+(d-1)\Lambda]C_\parallel'(R,t_1-t) + (\Lambda+1)RC_\parallel''(R,t_1-t)\Big]\Big|_{\boldsymbol{R}=\boldsymbol{x}_{t_1}^{(\mathrm{d})}-\boldsymbol{x}_t^{(\mathrm{d})}} \\
\boldsymbol{n}_0\cdot\langle \mathbb{A}(\boldsymbol{x}_t^{(\mathrm{d})},t)\boldsymbol{J}_{t_1}\rangle &= \langle B_{jk}(\boldsymbol{x}_{t_1}^{(\mathrm{d})},t_1)A_{ij}(\boldsymbol{x}_t^{(\mathrm{d})},t)\rangle n_{0,i}n_{0,k} - \langle B_{kl}(\boldsymbol{x}_{t_1}^{(\mathrm{d})},t_1)A_{ij}(\boldsymbol{x}_t^{(\mathrm{d})},t_1-t)\rangle n_{0,i}n_{0,j}n_{0,k}n_{0,l} \\
&= -\frac{1}{2R}\Big[(\Lambda-1)(d+1)C_\parallel'(R,t_1-t) - (\Lambda+1)RC_\parallel''(R,t_1-t)\Big]\Big|_{\boldsymbol{R}=\boldsymbol{x}_{t_1}^{(\mathrm{d})}-\boldsymbol{x}_t^{(\mathrm{d})}}
\end{aligned}
\tag{S16}
$$

### C. Results

Substituting the expressions derived in the previous Section into Eq. (S11) we obtain

$$
\begin{aligned}
\langle \boldsymbol{n}_t\cdot\boldsymbol{u}(\boldsymbol{x}_t,t)\rangle &= \mathrm{Ku}\int_0^t \mathrm{d}t_1\langle \boldsymbol{J}_{t_1}\cdot\boldsymbol{u}(\boldsymbol{x}_t^{(\mathrm{d})},t)\rangle + \mathrm{Ku}\,\Phi_\mathrm{s}\langle \boldsymbol{n}_0^\mathrm{T}\mathbb{A}(\boldsymbol{x}_t^{(\mathrm{d})},t)\int_0^t \mathrm{d}t_1(t-t_1)\boldsymbol{J}_{t_1}\rangle \\
&= \mathrm{Ku}\int_0^t \mathrm{d}t_1\,\frac{\boldsymbol{n}_0\cdot\boldsymbol{R}}{2R}\Big[[(d+1)+(d-1)\Lambda]C_\parallel'(R,t_1-t)+(\Lambda+1)RC_\parallel''(R,t_1-t)\Big]\Big|_{\boldsymbol{R}=\boldsymbol{x}_{t_1}^{(\mathrm{d})}-\boldsymbol{x}_t^{(\mathrm{d})}} \\
&- \mathrm{Ku}\,\Phi_\mathrm{s}\int_0^t \mathrm{d}t_1(t-t_1)\,\frac{1}{2R}\Big[(\Lambda-1)(d+1)C_\parallel'(R,t_1-t)-(\Lambda+1)RC_\parallel''(R,t_1-t)\Big]\Big|_{\boldsymbol{R}=\boldsymbol{x}_{t_1}^{(\mathrm{d})}-\boldsymbol{x}_t^{(\mathrm{d})}} \\
&= -d\Lambda\,\mathrm{Ku}\int_0^t \mathrm{d}t_1\;C_\parallel'(R,t_1-t)\Big|_{\boldsymbol{R}=\boldsymbol{x}_{t_1}^{(\mathrm{d})}-\boldsymbol{x}_t^{(\mathrm{d})}}\,,
\end{aligned}
\tag{S17}
$$

where we used $\boldsymbol{x}_t^{(\mathrm{d})} = \boldsymbol{n}_0 t$. Eq. (S17) is the dimensionless form of Eq. (4) in the Letter.

In the statistical model this expression can be evaluated further, owing to the fact that the (dimensionless) correlation function $C_\parallel(R,t)$ takes the simple form

$$
C_\parallel(R,t) = \frac{1}{d}e^{-R^2/2-|t|}\,. \tag{S18}
$$

in the statistical model [S4]. Inserting this expression into Eq. (S17) and assuming $\Phi_\mathrm{s} > 0$ yields

$$
\langle \boldsymbol{n}_t\cdot\boldsymbol{u}(\boldsymbol{x}_t,t)\rangle = \Lambda\,\mathrm{Ku}\,\Phi_\mathrm{s}\int_0^t \mathrm{d}t_1(t-t_1)e^{-\,\Phi_\mathrm{s}{}^2(t-t_1)^2/2-t+t_1} = \Lambda\,\mathrm{Ku}\,\Phi_\mathrm{s}\,\mathcal{H}\Big(\frac{1}{\sqrt{2}\,\Phi_\mathrm{s}}\Big) \tag{S19}
$$

Here we have defined $\mathcal{H}(x) \equiv 2x^2[1-\sqrt{\pi}xe^{x^2}\,\mathrm{erfc}(x)]$. Its asymptotes are

$$
\mathcal{H}(x) \sim 2x^2\left(1-\sqrt{\pi}x+2x^2-\sqrt{\pi}x^3+\frac{4}{3}x^4\right)+\dots\,,\ \text{for small } x\,, \tag{S20a}
$$

$$
\mathcal{H}(x) \sim 1-\frac{3}{2x^2}+\frac{15}{4x^4}-\frac{105}{8x^6}+\dots = \sum_{n=0}^{\infty}\frac{(-1)^n(2n+1)!!}{2^n x^{2n}}\,,\ \text{for large } x\,. \tag{S20b}
$$

Consequently, the small-$\Phi_\mathrm{s}$ behavior of Eq. (S19)) becomes

$$
\langle \boldsymbol{n}_t\cdot\boldsymbol{u}(\boldsymbol{x}_t,t)\rangle \sim \Lambda\,\mathrm{Ku}\,\Phi_\mathrm{s}\,, \tag{S21}
$$

which is the dimensionless form of Eq. (5) in the Letter. Eqs. (S19) and (S21) are specific to the statistical model with correlation function (S18). We note that Eq. (S19) is linear in $\Lambda$, and thus also Eqs. (S21). These results are obtained to order $O(\mathrm{Ku}^2)$. We expect that higher orders in Ku yield contributions that include higher orders in $\Lambda$, leading to deviations from linearity as $|\Lambda|$ increases, as observed in simulations (see Fig. 1a and Fig. 2 of the Letter).

In the main text we discuss the symmetries of the problem with respect to $\boldsymbol{n} \to -\boldsymbol{n}$. In the following we give the arguments in more detail. Swimming in the instantaneous direction $\boldsymbol{n}$ breaks the fore-aft symmetry of the problem. In other words, the dynamics of $\boldsymbol{n}$ is no longer invariant under $\boldsymbol{n} \to -\boldsymbol{n}$. This symmetry breaking is essential for the alignment bias described in the Letter and in this Supplemental Material. If the dynamics were invariant under $\boldsymbol{n} \to -\boldsymbol{n}$, then the expectation value $\langle \boldsymbol{u} \cdot \boldsymbol{n} \rangle$ would have to vanish. Yet, while fore-aft symmetry is broken, the equations of motion (S5a) and (S5b) are still invariant under $\boldsymbol{n} \to -\boldsymbol{n}$ and $\Phi_\mathrm{s} \to -\Phi_\mathrm{s}$. Taking $\boldsymbol{n} \to -\boldsymbol{n}$ in $\langle \boldsymbol{u} \cdot \boldsymbol{n} \rangle$ gives $\langle \boldsymbol{u} \cdot \boldsymbol{n} \rangle = -\langle \boldsymbol{u} \cdot (-\boldsymbol{n}) \rangle$. As a consequence $\langle \boldsymbol{u} \cdot \boldsymbol{n} \rangle$ must be an odd function of $\Phi_\mathrm{s}$. Note that it was assumed that $\Phi_\mathrm{s} > 0$ in the derivation of Eq. (S19). In general we have

$$\langle \boldsymbol{n}_t \cdot \boldsymbol{u}(\boldsymbol{x}_t, t) \rangle = \frac{\Lambda\,\mathrm{Ku}}{2\,{\Phi_\mathrm{s}}^2} \left\{ 2\,\Phi_\mathrm{s} - e^{1/(2\,{\Phi_\mathrm{s}}^2)} \sqrt{2\pi} \left[ \mathrm{erfc}\left( \frac{1}{\sqrt{2}\,\Phi_\mathrm{s}} \right) + \mathrm{sign}(\Phi_\mathrm{s}) - 1 \right] \right\} \tag{S22}$$

which is indeed odd in $\Phi_\mathrm{s}$ and simplifies to Eq. (S19) when $\Phi_\mathrm{s} > 0$. Note also that one obtains $\langle \boldsymbol{n}_t \cdot \boldsymbol{u}(\boldsymbol{r}_t, t) \rangle = 0$ for $\Lambda = 0$. In other words, rotational symmetry is recovered for spherical particles, and there is no alignment.

In the main text we briefly comment on the interpretation of the different mechanisms contributing to the observed alignment of $\boldsymbol{n}_t$ with $\boldsymbol{u}(\boldsymbol{x}_t, t)$. Here we give the details of the argument. To order $\mathrm{Ku}^0$ the swimmers have constant orientation $\boldsymbol{n} = \boldsymbol{n}_0$ and swim with constant swimming velocity $\Phi_\mathrm{s}\,\boldsymbol{n}_0$. To this order, trajectories are simply those of constant swimming, $\boldsymbol{r}_t = \boldsymbol{r}_0 + \Phi_\mathrm{s}\,\boldsymbol{n}_0 t$, and no alignment between the flow velocity $\boldsymbol{u}$ and the orientation $\boldsymbol{n}$ is observed. The first-order correction in Ku to the alignment between $\boldsymbol{u}$ and $\boldsymbol{n}$ in Eq. (S11) has two non-vanishing contributions:

$$\langle \boldsymbol{n}_t \cdot \boldsymbol{u}(\boldsymbol{x}_t, t) \rangle = \mathrm{Ku} \int_0^t \mathrm{d}t_1 \langle \boldsymbol{J}_{t_1} \cdot \boldsymbol{u}(\boldsymbol{x}_t^{(\mathrm{d})}, t) \rangle + \mathrm{Ku}\,\Phi_\mathrm{s} \langle \boldsymbol{n}_0 \cdot \mathbb{A}(\boldsymbol{x}_t^{(\mathrm{d})}, t) \int_0^t \mathrm{d}t_1 (t - t_1) \boldsymbol{J}_{t_1} \rangle\,.$$

The first contribution is due to changes in $\boldsymbol{n}$ (since $\boldsymbol{J}_t \propto \dot{\boldsymbol{n}}$), multiplied with the fluid velocity $\boldsymbol{u}$ evaluated along the straight deterministic $\mathrm{Ku}^0$-trajectory. The second contribution comes from a fixed orientation $\boldsymbol{n}_0$ times the difference $\boldsymbol{u}(\boldsymbol{x}_t, t) - \boldsymbol{u}(\boldsymbol{x}_t^{(\mathrm{d})}, t)$. This describes the consequence of the fact that the particles do not follow the deterministic trajectory, because $\boldsymbol{n}$ fluctuates. These two contributions depend upon the spatial dimension and $\Lambda$ in different ways. However, upon adding them, most terms cancel, leaving the relatively simple expression in Eq. (S13), proportional to $\Lambda$ and independent of the spatial dimension and compressibility of the underlying flow. It is possible that this cancellation is the result of a symmetry, but we have not yet found a simple argument.

## III. HIGHER MOMENTS $\langle (\boldsymbol{u}(\boldsymbol{x}_t, t) \cdot \boldsymbol{n}_t)^p \rangle$

Performing a similar expansion for the second moment $\langle (\boldsymbol{u}(\boldsymbol{x}_t, t) \cdot \boldsymbol{n}_t)^2 \rangle$ yields:

$$\langle (\boldsymbol{u}(\boldsymbol{x}_t, t) \cdot \boldsymbol{n}_t)^2 \rangle = \frac{1}{d} + \frac{\mathrm{Ku}^2\,\Lambda}{d} \left[ 2\mathcal{H}\Big( \frac{1}{\sqrt{2}\,\Phi_\mathrm{s}} \Big) - \mathcal{H}\Big( \frac{1}{\Phi_\mathrm{s}} \Big) + {\Phi_\mathrm{s}}^2 (d\Lambda - 1) \mathcal{H}\Big( \frac{1}{\sqrt{2}\,\Phi_\mathrm{s}} \Big)^2 \right]. \tag{S23}$$

The small-$\Phi_\mathrm{s}$ asymptote of this expression comes out as

$$\langle (\boldsymbol{u} \cdot \boldsymbol{n})^2 \rangle \sim \frac{1}{d} + \frac{\mathrm{Ku}^2\,\Lambda}{d} + \frac{\mathrm{Ku}^2\,{\Phi_\mathrm{s}}^2\,\Lambda}{2d} (2d\Lambda - 11)\,. \tag{S24}$$

Using corresponding results for higher-order moments allows us to compute the distribution of alignment between $\boldsymbol{u}$ and $\boldsymbol{n}_t$. To lowest order in Ku we find that the distribution of $u_n \equiv \boldsymbol{u}(\boldsymbol{x}_t, t) \cdot \boldsymbol{n}_t$ is simply a Gaussian with non-zero mean:

$$P(u_n) = \frac{1}{\sqrt{2\pi}\sigma} \exp\left[ -\frac{(u_n - \langle u_n \rangle)^2}{2\sigma^2} \right], \text{ with } \sigma = \frac{1}{\sqrt{d}}\,. \tag{S25}$$

Numerical statistical-model simulations show good agreement with this distribution when $\mathrm{Ku} = 0.1$ (not shown).

## IV. ALIGNMENT WITH VORTICITY

As briefly mentioned in the Letter, previous results (see Ref.[14,31] of the Letter) have shown that for elongated ($\Lambda > 1$) swimmers moving in a turbulent flow there is a nematic-like alignment, i.e. the cos of the angle, $\theta_\omega$, between $\boldsymbol{n}$ and $\boldsymbol{\omega}$ tends to assume values $\pm 1$. Here, for the sake of completeness, in Fig. 1, we show that indeed while $\langle \cos\theta_\omega \rangle = 0$ for any swimming number and shape parameter, the second moment displays a nontrivial $\Lambda$ dependence. In particular, it becomes larger than 1/3 (the value for uniformly distributed orientations) when $\Lambda \to 1$. Moreover, there is a weak dependence on the swimming speed, and its values are basically the same of those of non-swimming particles, i.e. also non-swimming particles tend to be nematically ordered with respect to the underlying velocity field. Conversely, disks tend to be more and more oriented orthogonally to the vorticity as $-\Lambda$ grows, leading to values smaller than 1/3. As discussed in Ref. [27] of the Letter, this alignment, at least for rods can be traced back to a dynamical effect due to the similarity between the equation for $\boldsymbol{n}$ and that of the vorticity in the Lagrangian frame. Indeed, for rod shaped tracers ($\Lambda = 1$) in turbulence, Eq. (S5b) for the orientation reduces to $\dot{\boldsymbol{n}} = \mathbb{A}\boldsymbol{n} - (\boldsymbol{n}\cdot\mathbb{A}\boldsymbol{n})$ that is formally similar to the Lagrangian dynamics of the vorticity, $\dot{\boldsymbol{\omega}} = \mathbb{A}\boldsymbol{\omega} - \nu\Delta\boldsymbol{\omega}$. While, as reported in Ref. [27], for tracer particles in stochastic flows similar to those discussed here there is no such alignment. In the following we show that this can be proved to be the case also for swimming particles in our statistical model.

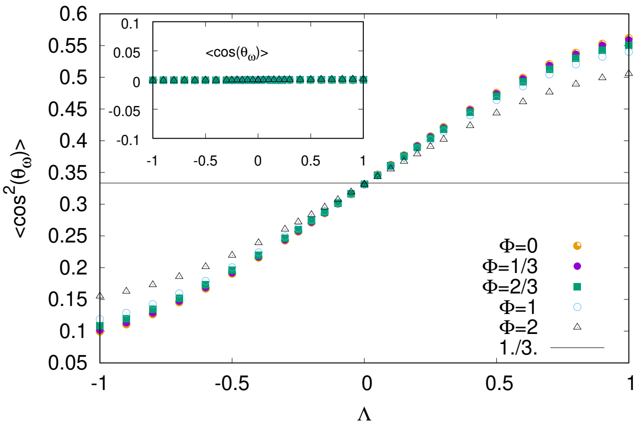


FIG. 1: (Color online) Statistics of particle orientation with respect to vorticity, obtained from direct numerical simulations of the Navier-Stokes equations at $Re_\lambda \approx 68$, as a function of the particle shape parameter $\Lambda$, for different swimming number $\Phi = v_s/u_\eta$ as in legend. Main panel shows $\langle \cos^2\theta_\omega \rangle$; the inset shows $\langle \cos\theta_\omega \rangle$. Statistics computed as in Fig.1 of main text.

The average alignment between vorticity, $\boldsymbol{\omega}(\boldsymbol{x}_t, t) = \boldsymbol{\nabla} \wedge \boldsymbol{u}(\boldsymbol{x}_t, t)$, and $\boldsymbol{n}_t$, $\langle \boldsymbol{\omega}(\boldsymbol{x}_t, t)\cdot\boldsymbol{n}_t \rangle = \epsilon_{ijk}\langle O_{kj}(\boldsymbol{x}_t, t) n_{t,j}\rangle$ ($O_{ij}$ being the entries of the antisymmetric component of the velocity gradients) must vanish by symmetry. In fact all odd moments of $\boldsymbol{\omega}\cdot\boldsymbol{n}_t$ must evaluate to zero. This can be seen as follows. The index structure of any expansion of the steady-state average $(\langle O_{kj} n_{t,i})^{2p+1}\rangle$ to any order in Ku can be expressed as sums over correlation functions of the fluid. For an isotropic flow, the correlation functions are proportional to products of Kronecker delta symbols, $\delta_{ij}$. They cannot contain the Levi-Civita tensor, $\epsilon_{ijk}$, unless parity invariance is broken. As a consequence, the average $\langle (O_{kj} n_{t,i})^{2p+1}\rangle$ must vanish in the steady state, since it has an odd number of indices. It follows that $(\langle O_{kj} n_{t,i})^{2p+1}\rangle$ must vanish. Even moments, by contrast, have an even number of indices and are therefore in general non-zero. In the statistical model the second moment has a vanishing correction to order $\mathrm{Ku}^2$:

$$\langle (\boldsymbol{\omega}(\boldsymbol{x}_t, t)\cdot\boldsymbol{n}_t)^2 \rangle = \frac{20}{3} + O(\mathrm{Ku}^3)\,.$$

We emphasize that this result demonstrates that the alignment observed in fig. 1 has a *dynamical origin.*

## V. AVERAGE ALIGNMENT FOR TURBULENT FLOWS

In this Section we briefly explain how Eq. (6) of the Letter was derived and show its validity also for the statistical model. Equation. (S17) was derived for the statistical model in the limit of small values of Ku. It expresses the average alignment in terms of a time integral over an Eulerian correlation function. More generally, if we neglect the effect of the rotational part $\mathbb{O}$ upon the orientation dynamics, we can expand the average alignment in terms of small swimming speed $v_\mathrm{s}$ and small shape factor $\Lambda$ around Lagrangian trajectories, similar to the expansion in Ref. [S7].

We find (in dimensional units)

$$\langle \boldsymbol{n}_t \cdot \boldsymbol{u}(\boldsymbol{x}_t, t)\rangle = \frac{2\Lambda v_{\rm s}}{d+2}\int_0^t {\rm d}t_1 t_1\, {\rm Tr}\langle \mathbb{S}(\boldsymbol{x}_{t_1}^{(\rm L)}, t_1)\mathbb{S}(\boldsymbol{x}_0^{(\rm L)}, 0)\rangle\,. \tag{S26}$$

Here $\mathbb{S}(\boldsymbol{x}_{t_1}^{(\rm L)}, t_1)$ is the fluid strain evaluated along a Lagrangian trajectory, $\boldsymbol{x}_t^{(\rm L)}$, following the dynamics $\dot{\boldsymbol{x}}_t^{(\rm L)} = \boldsymbol{u}(\boldsymbol{x}_t^{(\rm L)}, t)$. As check, we numerically evaluated the Lagrangian correlation function ${\rm Tr}\langle \mathbb{S}(\boldsymbol{x}_{t_1}^{(\rm L)}, t_1)\mathbb{S}(\boldsymbol{x}_0^{(\rm L)}, 0)\rangle$ for the statistical model with ${\rm Ku} = 1$ and numerically computed the integral in Eq. (S26) obtaining $\approx 0.625$. Then we evolved swimming particles with different shapes for two values of $v_s$ and computed $\langle \boldsymbol{n}\cdot\boldsymbol{u}\rangle$. In Fig. 2 we show that indeed $(d+2)/2\langle \boldsymbol{n}\cdot\boldsymbol{u}\rangle$ agrees well with the prediction $0.625\Lambda$. We emphasize that Eq. (S26) assumes that the swimming speed $v_{\rm s}$ and the shape factor $\Lambda$ are small, and that the effect of $\mathbb{O}$ is negligible, but makes no further assumption about the nature of the flow. Eq. (S26) is compared to results from DNS of homogeneous isotropic turbulence in Fig.3b of the Letter, where a very good agreement is also found.

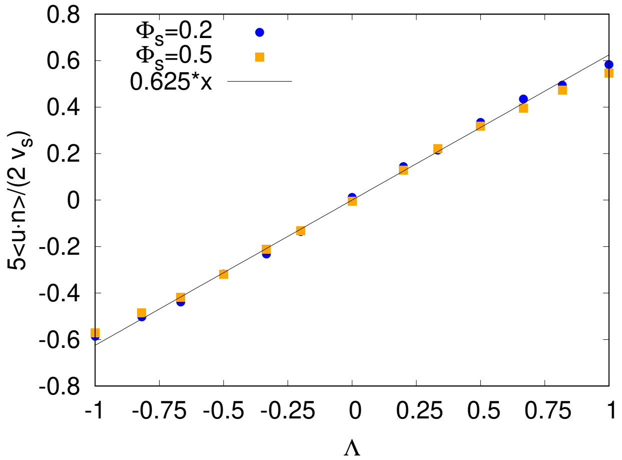


FIG. 2: (Color online) Check of the validity of Eq. (S26) for the statistical model at ${\rm Ku} = 1$. The plot shows $5\langle(n\cdot u)\rangle/(2v_s)$ vs $\Lambda$ for two swimming speeds. The solid line represents the prediction Eq. (S26), namely $0.625\Lambda$, obtained by numerically evaluating the integral as described in the text.

A further check of the above prediction is obtained by making a small $\Phi_{\rm s}$ expansion of Eq. (S17). This gives (in dimensional units)

$$\langle \boldsymbol{n}_t \cdot \boldsymbol{u}(\boldsymbol{x}_t, t)\rangle \sim -d\Lambda v_{\rm s}\int_0^t {\rm d}t_1 (t-t_1)\partial_R^2 C_\parallel(0, t-t_1) = \frac{2\Lambda v_{\rm s}}{(d+2)}\int_0^t {\rm d}t_1 t_1\, {\rm Tr}\langle \mathbb{S}(0, t_1)\mathbb{S}(0,0)\rangle\,. \tag{S27}$$

The only difference between the small Ku expansion Eq. (S27) and the general result Eq. (S26) is that the latter is evaluated using Lagrangian statistics while the former is evaluated using Eulerian statistics. This is not in contradiction, to lowest order in Ku the two statistics coincide.

[S1] E. Calzavarini, R. Volk, M. Bourgoin, E. Leveque, J. F. Pinton, and F. Toschi. Acceleration statistics of finite-sized particles in turbulent flow: the role of Faxén forces. *J. Fluid Mech.*, 630:179, 2009.
[S2] G. Falkovich, K. Gawedzki, and M. Vergassola. Particles and fields in fluid turbulence. *Rev. Mod. Phys.*, 73:913–975, 2001.
[S3] U. Frisch. *Turbulence*. Cambridge University Press, Cambridge, UK, 1997. 296p.
[S4] K. Gustavson and B. Mehlig. Statistical models for spatial patterns of heavy particles in turbulence. *Adv. Phys.*, 65:1, 2016.
[S5] K. Gustavsson and B. Mehlig. Ergodic and non-ergodic clustering of inertial particles. *Europhys. Lett.*, 96:60012, 2011.
[S6] K. Gustavsson, M. Z. Sheikh, D. Lopez, A. Naso, A. Pumir, and B. Mehlig. Theory for the effect of fluid inertia on theorientation of a small spheroid settling in turbulence. *arxiv:1904.00481*, 2019.
[S7] S. Vajedi, K. Gustavsson, B. Mehlig, and L. Biferale. Inertial-particle accelerations in turbulence: a Lagrangian closure. *J. Fluid Mech.*, 798:187–200, 2016.
